# Supplementary material for: "Newspaper Eat" Means "Not Tasty": A Taxonomy and Benchmark for Coded Language in Real-World Chinese Online Reviews
Source: arXiv:2601.19932 source file (2026-04-22)
Supplement: Supplementary file 1 [file additional_classification.tex]

\begin{table}[t]
\centering
\small
\begin{tabular}{lcccc}
\toprule
\textbf{Coded Language Class} & \textbf{P} $\uparrow$ & \textbf{R} $\uparrow$ & \textbf{F1} $\uparrow$  \\
\midrule
Ambiguous Homophone        & 0.66 & 0.61 & 0.63  \\
Non-Lexical Homophone      & 0.65 & 0.54 & 0.59  \\
Phonetic Substitution      & 0.50 & 0.95 & 0.65  \\
Emoji Substitution         & 0.75 & 0.25 & 0.38 \\
Cipher                     & 0.86 & 0.81 & 0.84 \\
Orthographic Substitution  & 0.30 & 0.91 & 0.45  \\
Cross-Lingual Phonetic Encoding & 0.05 & 1.00 & 0.10  \\

\bottomrule
\end{tabular}
\caption{Per-class coded language classification performance for \texttt{GPT-5-mini}.}
\label{tab:gpt_classification}
\end{table}

\begin{table}[t]
\centering
\small
\begin{tabular}{lccc}
\toprule
\textbf{Coded Language Class} & \textbf{P} $\uparrow$ & \textbf{R} $\uparrow$ & \textbf{F1} $\uparrow$  \\
\midrule
Ambiguous Homophone & 0.57 & 0.61 & 0.59 \\
Non-Lexical Homophone & 0.68 & 0.73 & 0.70 \\
Phonetic Substitution & 0.51 & 0.97 & 0.67\\
Emoji Substitution & 0.77 & 0.83 & 0.80  \\
Cipher & 0.78 & 0.85 & 0.81 \\
Orthographic Substitution & 0.46 & 0.97 & 0.63 \\
Cross-Lingual Phonetic Encoding & 0.04 & 1.00 & 0.08 \\
\bottomrule
\end{tabular}
\caption{Per-class coded language classification performance for \texttt{Gemini-2.5-Flash}.}
\label{tab:gemini_classification}
\end{table}

\begin{table}[t]
\centering
\small
\begin{tabular}{lccc}
\toprule
\textbf{Coded Language Class} & \textbf{P} $\uparrow$ & \textbf{R} $\uparrow$ & \textbf{F1} $\uparrow$ \\
\midrule
Ambiguous Homophone & 0.45 & 0.23 & 0.30 \\
Non-Lexical Homophone & 0.38 & 0.30 & 0.34 \\
Phonetic Substitution & 0.48 & 0.16 & 0.24 \\
Emoji Substitution & 0.10 & 0.08 & 0.09 \\
Cipher & 0.45 & 0.12 & 0.19 \\
Orthographic Substitution & 0.17 & 0.65 & 0.27 \\
Cross-Lingual Phonetic Encoding & 0.09 & 0.57 & 0.16 \\
\bottomrule
\end{tabular}
\caption{Per-class coded language classification performance for \texttt{Qwen2.5-7B-Instruct}.}
\label{tab:qwen_classification}
\end{table}
